# Supplementary material for: Characteristics of Four Upward-pointing Cosmic-ray-like Events Observed with ANITA
Source: arXiv:1603.05218 source file (2016-06-29)
Supplement: Supplementary file 1 [file anita-upshowers-rev10-suppl.pdf]

## Supplemental Materials for *Characteristics of Four Upward-pointing Cosmic-ray-like Events Observed with ANITA*

### ANITA-I AND ANITA-II FLIGHT SUMMARY.

The original ANITA-I flight, which took place in the Antarctic austral summer of 2006-2007, has been described in detail elsewhere [S1]. ANITA-I flew 32 dual-polarized quad-ridged horns in two azimuthal rings separated vertically by about 3 m. The rings were arranged in 16 azimuthal sectors separated by  $22.5^\circ$ , so that two antennas observed the same field of view, with a beam size of order  $40^\circ$  angular diameter, thus overlapping with the adjacent azimuthal sectors. Hpol and Vpol signals were converted to LCP and RCP, and a multi-antenna coincidence was formed for impulses above a threshold of a few times the thermal noise. This trigger was thus blind to the plane-of-polarization, and as a result was equally efficient in detecting the cosmic rays, which were predominantly Hpol due to the Antarctic geomagnetic field, and Vpol or mixed-polarization signals, as long as they had a high degree of linear polarization.

ANITA-II, which flew in the austral summer of 2009-2010, did not use the LCP+RCP combination, since it causes some loss of sensitivity if the expected signals are close to alignment with the antenna polarization vector. This was expected to be the case for neutrino signals arising from the Askaryan effect within the ice sheet, due to Fresnel effects at the surface. To optimize neutrino sensitivity, and for cost reasons, ANITA-II's trigger used only the vertically polarized signals directly, since at the time the cosmic-ray detection channel was not fully understood, and was deemed of only secondary interest. Thus ANITA-II could only detect CRs through their residual vertically polarized component, which is generally small in Antarctica because of the nearly vertical magnetic field.

Both payloads flew at similar altitudes, typically 35-38 km depending on the time of day and the ambient stratospheric temperature. The horizon from these altitudes is depressed below the horizontal to about  $-6.5^\circ$ , and both payloads could trigger and reconstruct event locations effectively down to about  $-40^\circ$ , covering the vast majority of the ice surface in view.

### PROBABILITY ANALYSIS DETAILS.

Event D in our sample is entirely excluded as arising from a fluctuation in the radio thermal noise background. Its raw signal is evident in multiple antennas, and its coherence and polarization properties are too singular to be mimicked by a fluctuation within the range of the ANITA-I flight exposure. It is thus either of anthropogenic origin, or a cosmic-ray air shower. To estimate the chance probability (or  $p$ -value) that event D is a statistical fluctuation of the anthropogenic background we have investigated the distributions of various parameters of the background sample as compared to those observed for event D, as summarized in the main text. We provide details of that analysis here.

#### Correlation to UHECR pulse shape

Fig. S1 shows a two-dimensional histogram of the correlation coefficients for the observed waveforms and the instrumental-deconvolved waveforms for the  $\sim 80,000$  anthropogenic signals observed by ANITA-I. The events are correlated with the average observed and instrumentally-deconvolved waveforms of the 14 reflected UHECR events from ANITA-I. The correlation coefficients of the 14 reflected and two non-reflected (above-horizon) events are also shown.

In the initial unblinding analysis which led to the first CR sample, event correlation coefficients and delays within the sample window were determined by choosing the highest values in the cross-correlation without checking against possible high sidelobes due to noise fluctuations. Thus event D's precise time delay within the window was inadvertently assigned to a sidelobe lag, leading to an incorrect polarity, and apparent agreement in polarity with the existing reflected CRs. Later analysis discovered this delay offset, and, once it is corrected, the polarity is found to be inverted with respect to the reflected CRs. We plot both values in Fig. S1. To estimate the normalized probability of an anthropogenic event equaling or exceeding the correlation value of event D, we thus integrate the regions shown in Fig. S1, accounting for the additional trial of either polarity (due to the original method), by integrating both the correlated and anti-correlated possibility. The result is that 2.2% of the cumulative event coefficients exceed the coefficient for event D.

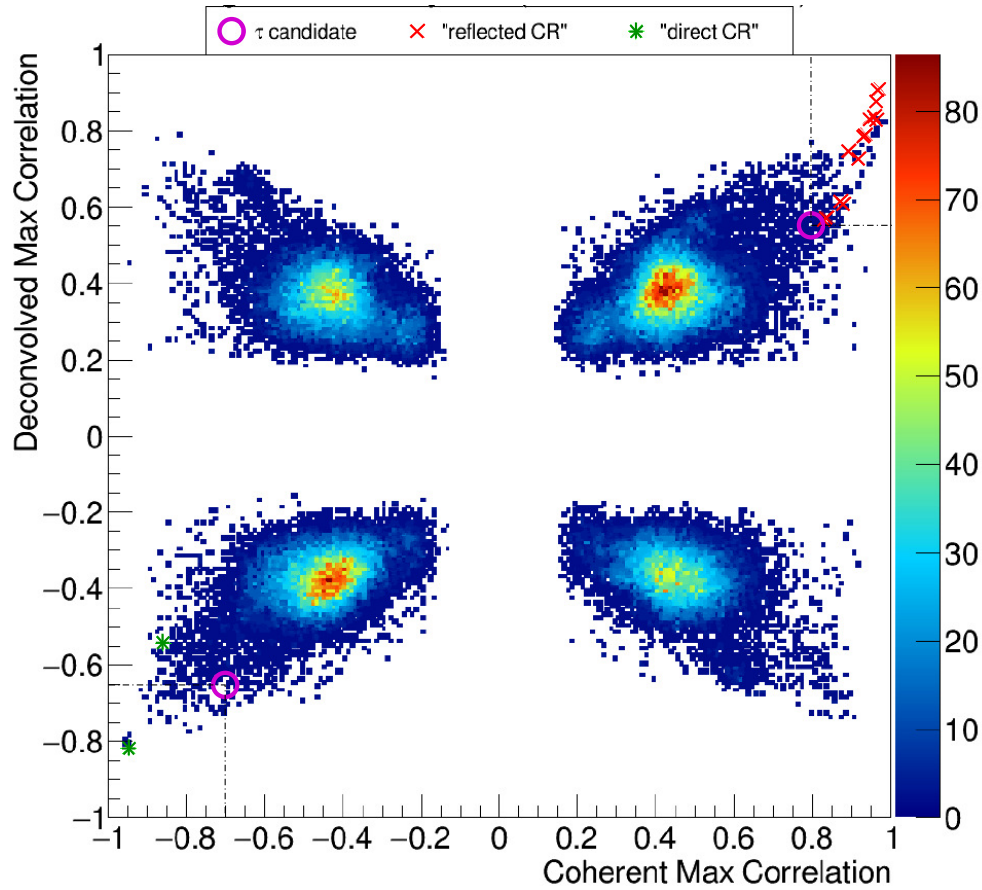

FIG. S1: The observed distribution of the normalized correlation coefficient of about 80,000 events of predominantly anthropogenic origin from the ANITA-I flight with the average pulse shape of the 14 established UHECR events [S2]. Event D (magenta circle) is plotted twice, for both the positive correlation (with incorrect group delay) and anti-correlation, with correct group delay, but inverted phase relative to the reflected CRs.

### Polarity analysis

Clearly, the delay offset mentioned above indicates that, unless care is taken to ensure that the polarity is measured at the correct delay, it can be estimated incorrectly. Thus we undertook extensive investigations of our estimation of polarity, and we find that, at the signal-to-noise ratio of the observed CR events, the possibility of mistakes in polarity is negligible.

In Fig. S2 we show deconvolved waveforms for all 18 of the CRs discussed here, annotated by their event numbers, including the 3 above-horizon events and event D. To estimate the cross-correlation coefficients accurately, and thus determine the polarity, the waveforms are aligned by matching delays to the zero-crossing of the central bipolar signal, a process that is unambiguous in all of the cases we have considered. To produce normalized cross-covariance (statistically very similar to the cross-correlation) we remove any DC bias in any waveform, and normalize the resulting coefficients using the auto-covariance values.

To illustrate the robustness of the polarity estimates we produce here a cross-covariance estimate for each CR waveform with every other waveform of the ensemble. The cross-covariance coefficients so determined are plotted as a matrices in Figure S3. The left is the case where the reference waveforms, each of the reflected CRs in this case, are not inverted. It is evident that the CRs are highly correlated to each other, but anti-correlated to the above-horizon CRs (indices 12,16,18), and to event D (index 9). These four latter events all do correlate well with each other. On the right is the complementary case where now the 14 original reflected CRs are each inverted relative to their original polarity before they are cross-correlated. This shows that their inverted form correlates well with the above-horizon events, and with event D.

Fig. S4 shows a histogram of the cross-covariance values from Fig S3. It is evident that event D lies on the edge of the distribution with regard to its covariance values, but is still within the plausible envelope of the distribution. It is also evident that the overlap in the distributions between the covariant and contra-variant sides is negligible, indicating that the chance of misidentified polarity for these events is very small.

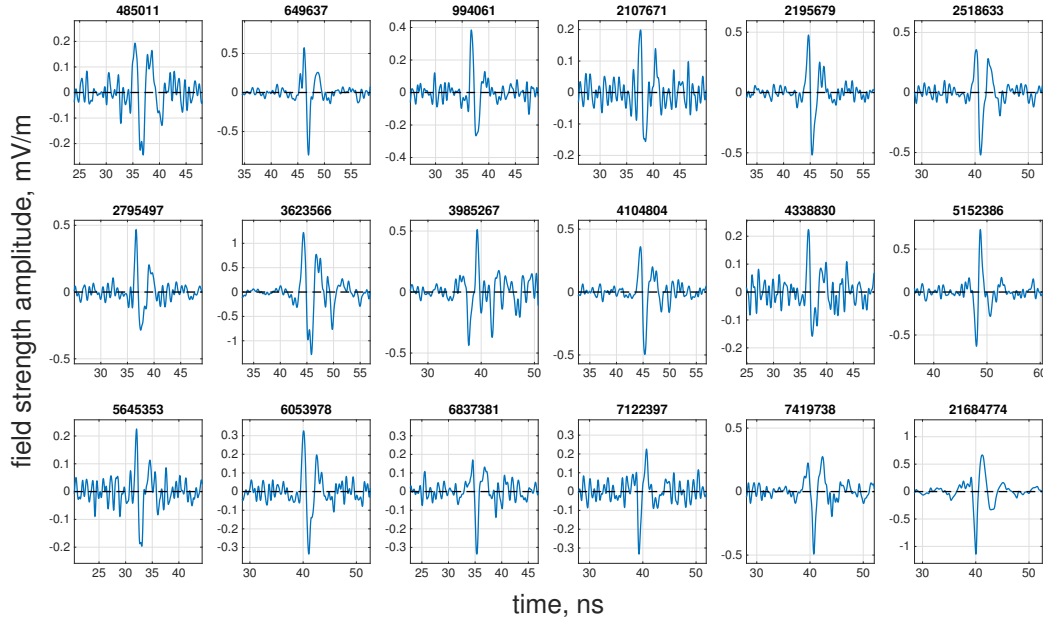

FIG. S2: Deconvolved, coherently-summed waveforms for all 18 of the CRs, along with event D, discussed in the main text.

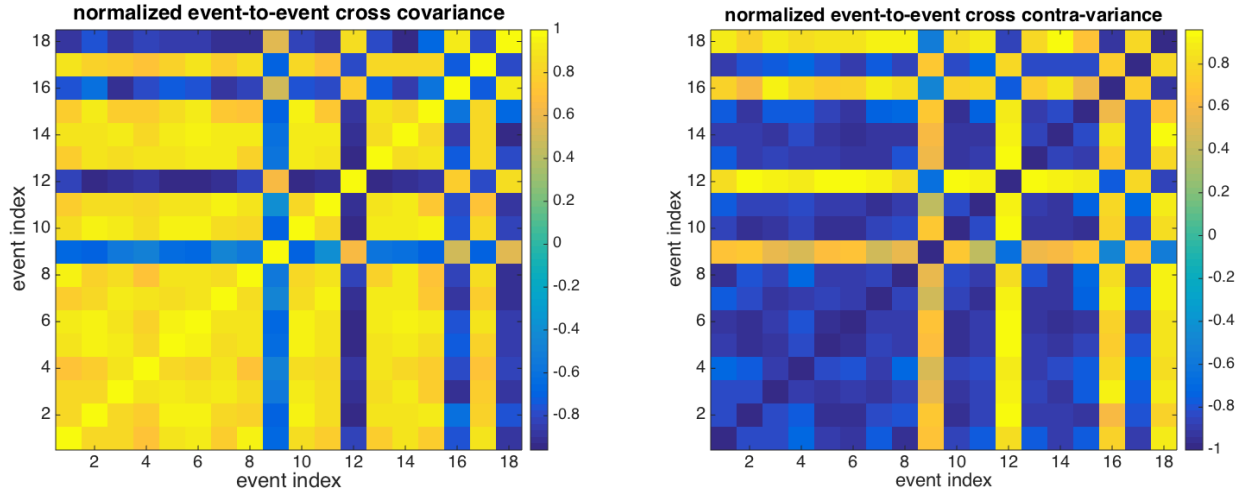

FIG. S3: Normalized cross-covariance of the 18 CRs against each other (left), and (right) the same plot except that each reflected CR is inverted before the correlation. Event indices are based on the location in Fig. S2, numbering sequentially from upper left to lower right.

### Geomagnetic chance alignment.

For ANITA-I, each set of H and V antenna signals was first converted to left and right-circular polarization (LCP and RCP) prior to triggering the payload. This was done to ensure that each signal had a high degree of linear polarization (LP), as expected from the physics signals ANITA was designed to detect. Signals that have 100% LP produce equal amplitudes in both LCP and RCP, and ANITA's trigger required a coincidence between LCP and RCP to trigger. This also meant that the trigger was blind to the plane of polarization of a LP impulse.

To estimate the chance that a random anthropogenic trigger would have a plane-of-polarization that matched the expected plane of polarization for a CR shower, given the local geomagnetic parameters of Antarctica, we looked at a distribution of 2155 anthropogenic Hpol-dominant ANITA events. Of these, 160 had values equal to or closer to the expected values than event D,

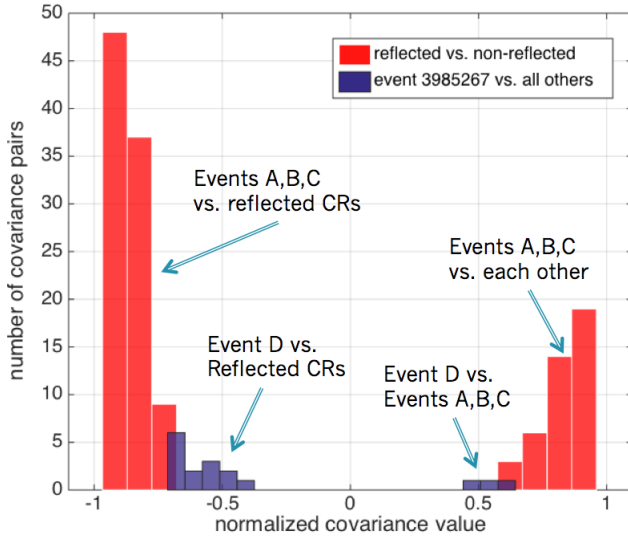

FIG. S4: Histogram of the cross-covariance values from Fig S3.

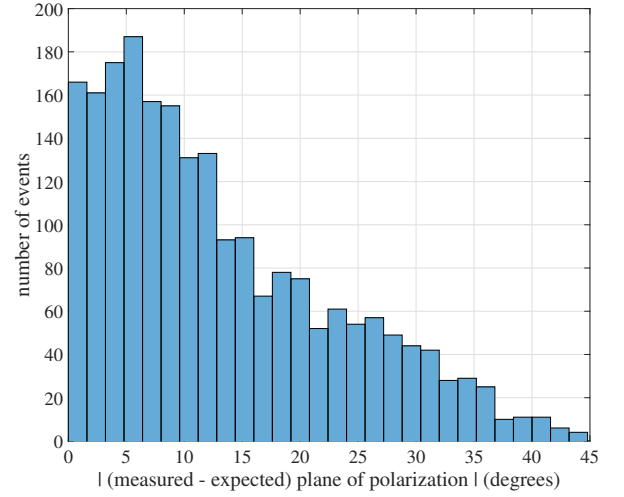

FIG. S5: Histogram of the expected vs. measured planes of polarization for a set of ANITA Hpol-dominant anthropogenic events.

giving a  $p$ -value of 0.07. Fig. S5 shows a histogram of these values. The distribution is non-uniform primarily because the geomagnetic field in Antarctica favors the vertical direction.

#### Stokes V chance probability.

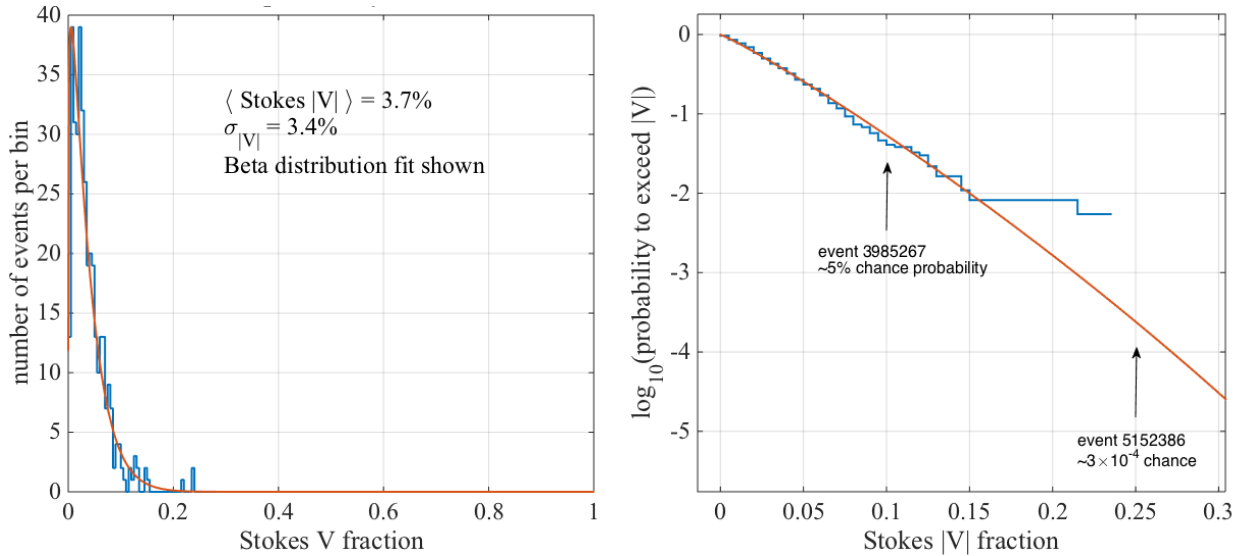

FIG. S6: Left: distribution of instrumental Stokes V content in  $\sim 400$  ground-to-payload pulses measured for ANITA-I. Right, the cumulative probability for this distribution, with event D and event A marked.

Although circular polarization (CP) is ubiquitous in VHF-UHF satellite-to-ground communications because of the challenges of transmission through the ionosphere, it is not commonly used in Antarctic surface installations, and is thus relatively rare in anthropogenic impulses seen from Antarctic surface locations. However, CP can be produced in linearly-polarized signals via spurious instrumental response, and we find this to be an important source of potential background CP in our data. To estimate this instrumental contamination, we carefully measured the Stokes V content of  $\sim 400$  horizontally-polarized ground-to-payload calibration impulses recorded during ANITA-I.

The distribution of the magnitude of Stokes V (which measures the CP content) is shown in Fig. S6(Left). This follows closely the expected  $\beta$ -distribution of a random bounded quantity. In the right figure, we show the cumulative distribution and marked positions for events D and A. Spurious values of Stokes V greater than event D in horizontally-polarized events occur about 5% of the time.

### ANGULAR UNCERTAINTY ESTIMATE & CHORD LENGTH.

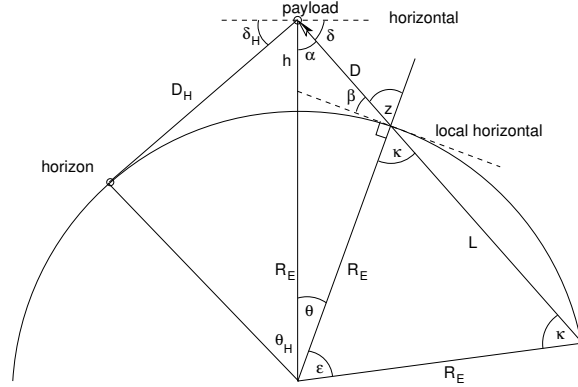

FIG. S7: Geometry for the possible emergence of event D from the Earth.

The estimates of angular uncertainty for the emergence angle of event D arise from two sources: first, the statistical uncertainty in our estimate of the arrival direction of the radio signal, which is about  $0.3^\circ$  in this case, and has been extensively verified using in-flight ground-to-payload radio pulsers [S1]. Second, radio emission from an air shower is now believed to develop into a hollow conical beam in the far field, with an angular radius of order  $1^\circ$  [S3].

Since we have no way to constrain what part of this ring we might be observing, it thus forms a systematic error that is convolved with the statistical error on the direction of the CR shower. In this case, assuming that a putative  $\tau$ -lepton is closely aligned to its parent neutrino direction, and accounting for the curvature of the Earth, we arrive at a minimum emergence angle, relative to the surface, of  $25.4^\circ$ , which in turn then defines the chord through the Earth that must be integrated to determine the column density.

Fig. S7 shows the geometry for a ray through the earth arriving at the payload. The payload is at altitude  $h$ , typically 35-38 km. The horizon is at a local elevation angle of  $\delta_H$  below the horizontal at the payload. The event arriving along the chord  $L$  through the Earth emerges at zenith angle  $z$  and local elevation angle  $\beta$  relative to the surface tangent at that location, which is distance  $D$  from the payload, at a nadir angle  $\alpha$  and elevation angle  $\delta$ . From this,  $\sin\theta = D\cos\delta/R_E$  and  $D^2 = R_E^2 + (R_E + h)^2 - 2R_E(R_E + h)\cos\theta$ . The emergence angle of the track (the elevation angle relative to the local surface tangent) is then  $\beta = \delta - \theta$  and the chord length  $L$  is given by  $L = 2R_E \sin\beta$ , which for a polar earth radius  $R_E = 6356.8$  km, gives  $L = 5450$  km.

In determining the resulting column density for this chord, a shell-model of the Earth was numerically integrated, including different appropriate densities for the ice, crust, mantle, and core. Standard model cross sections per nucleon for neutrino interactions were used, giving typical values for the charged current cross section of  $\sim 2 \times 10^{-32}$  cm<sup>2</sup> per nucleon at 1 EeV. In the main text above we have standardized the interaction lengths in km of water-equivalent mass, thus normalizing to the density of water, although only a small portion of the track is in ice or water. Since a large portion of the chord passes through the mantle, its average density along the track is of order  $3.7$  gm cm<sup>-3</sup>, thus at 1 EeV, the average interaction length is of order  $L_{int} = 440$  km, from which the overall attenuation  $A$  follows from  $A = \exp(-L/L_{int})$ .

[S1] Gorham, P. W. *et al.*, *Astropart. Phys.* **32**, 10-41 (2009).

[S2] S. Hoover, unpublished PhD. dissertation, UCLA, 2010.

[S3] H. Schoorlemmer, *et al.*, [ANITA collaboration], *Astropart. Phys.* (2016, in press; also arXiv:1506.05396).
